# Supplementary material for: SoftCache: Adaptive Step Size Caching for Diffusion Transformers
Source: arXiv:2610.22369 source file (2026-10-15)
Supplement: Supplementary file 1 [file crop.tex]

% Generated by paper_data/figures/supp_grid_flux/build_manifest.py -- do not edit.
\def\zboxx{0.546875}\def\zboxy{0.410156}\def\zboxs{0.312500}
